# Supplementary material for: Stochastic Deep Networks
Source: arXiv:1811.07429 source file (2019-02-20)
Supplement: Supplementary file 1 [file appendix.tex]

% !TEX root = ../StochasticDeepAISTATS20019.tex

%%%%%%%%%%%%%%%%%%%%%%%%%%%%%%%%%%%%%%%%%%%%%%%%%%%%%%%%%
%%%%%%%%%%%%%%%%%%%%%%%%%%%%%%%%%%%%%%%%%%%%%%%%%%%%%%%%%
%%%%%%%%%%%%%%%%%%%%%%%%%%%%%%%%%%%%%%%%%%%%%%%%%%%%%%%%%
\section{Useful Results}

This section recaps important results on measure spaces and Wasserstein distances.
