# Supplementary material for: Stochastic Deep Networks
Source: arXiv:1811.07429 source file (2019-02-20)
Supplement: Supplementary file 2 [file suppl-aux.tex]

\section{Building Blocks on Measures} \label{building-blocks-measures}

In this section are presented proved regularity properties of building blocks that are used in the main sections, all rephrased in terms of measures.

\paragraph{Notations} 
If $\Xx$ is a metric space, with associated distance $d_\Xx$, $\Mm_+^1(\Xx)$ is the space of (Radon) probability measure. 
%
We denote $\Cc(\Xx)$ the space of continuous functions from $\Xx$ to $\RR$. 
%
For two metric spaces $(\Xx,\Yy)$, we denote $\Cc(\Xx;\Yy)$ the space of continuous functions from $\Xx$ to $\Yy$. 

%%%%%%%%%
\paragraph{1-Wasserstein distance.} 

The $1$-Wasserstein distance, denoted $\Wass_{\Xx}$, is

\eq{
	\begin{split}
	\foralls (\mu,\nu) \in \Mm_+^1(\Xx)^2, & \quad \\
	\Wass_{\Xx}(\mu,\nu) \eqdef & \umin{\pi \in \Pi(\mu,\nu)} \int_{\Xx \times \Xx} d_\Xx(x,y) \d\pi(x,y). \\
	\end{split}
}
where
\eq{
	\Pi(\mu,\nu) \eqdef \enscond{\pi \in \Mm(\Xx \times \Xx)}{ P_{1,\sharp}\pi=\mu, P_{2,\sharp}\pi=\nu }.
}
Note that $\Wass_{\Xx}$ is a norm, and can be conveniently computed using
\eq{
	\Wass_{\Xx}(\mu,\nu) = \Wass_{\Xx}(\mu-\nu) = \umax{\Lip(g) \leq 1} \int_\Xx g \d(\mu-\nu).
}

%%%%%%%%%
\paragraph{Continuity.} 

Recall that a map $T : \Mm(\Xx) \rightarrow \Mm(\Yy)$ is weak-$*$ continuous if for any continuous $\phi$, $\int \phi \d\mu_k \rightarrow \int \phi \d\mu$ implies $\int \phi \d T(\mu_k) \rightarrow \int \phi \d T(\mu)$. Equivalently, if $\Wass_\Xx(\mu_k,\mu) \rightarrow_k 0$ then $\Wass_\Yy(T(\mu_k),T(\mu)) \rightarrow_k 0$. 
%
Such a map is said to be $C$-Lipschitz for the Wasserstein distance if 
\eq{
	\foralls (\mu,\nu) \in \Mm(\Xx)^2, \quad
	\Wass_\Yy( T(\mu),T(\nu) )
	\leq 
	C \, \Wass_\Xx( \mu,\nu ).
}

In this context, let us review main operations on measures used in section \ref{sec:description} and analyze regularity of our elementary block.

%%% Push-forward.
\paragraph{\underline{Push-forward.}} The push-forward block allows for modifications of the support while maintaining the geometry of the input measure.
\begin{defn}[Push-forward]
For a function $f : \Xx \rightarrow \Yy$, we define the push-forward  $f_\sharp \mu \in \Mm(\Yy)$ of $\mu \in \Mm(\Xx)$ by $T$ as defined by
\eql{\label{eq-push-foward}
	\foralls g \in \Cc(\Yy), \quad 
	\int_\Yy g \d(f_\sharp \mu) \eqdef \int_\Xx g(f(x)) \d\mu(x).	
}
\end{defn}
\noindent Note that $f_\sharp : \Mm(\Xx) \rightarrow \Mm(\Yy)$ is a linear operator. 


\begin{prop}[Lipschitzness of push-forward]\label{prop-lip-pushforward}
	One has 
	\begin{align}
		\Wass_\Yy(f_\sharp \mu,f_\sharp \nu) &\leq \Lip(f) \Wass_\Xx(\mu,\nu), \label{lip_push_1} \\
		\Wass_\Yy(f_\sharp \mu,g_\sharp \mu) &\leq \norm{f-g}_{L^1(\mu)} \label{lip_push_2}
	\end{align}
	where $\Lip(f)$ designates the Lipschitz constant of $f$.
\end{prop}

\begin{proof}
$\forall h$ s.t. $\Lip(h) \leq 1, \frac{h \circ f}{\text{Lip}(f)}$ is 1-Lipschitz, therefore
$$ \int_\Xx \frac{h \circ f}{\Lip(f)} \mathrm{d}(\mu-\nu) \leq \Wass_\Xx(\mu,\nu)
$$
hence inequality (\ref{lip_push_1}). Similarly, $\forall h$ s.t. $\Lip(h) \leq 1,$
$$ \int_\Xx (h \circ f - h \circ g) \mathrm{d}\mu \leq \int_\Xx \norm{f(x)-g(x)}_{\Yy} \mathrm{d}\mu(x) $$
hence inequality (\ref{lip_push_2}).
\end{proof}

%%% Tensorization.
\paragraph{\underline{Tensorization.}}
Tensorization plays an important role to densify input measures while generating interactions between input points.
\begin{defn}[Tensor product]
For $(\mu,\nu) \in \Mm(\Xx) \times \Mm(\Yy)$, $\mu \otimes \nu \in \Mm(\Xx \otimes \Yy)$ is the tensor product measure, defined for any continuous function $g : \Xx \times \Yy \rightarrow \RR$ as
\eq{
	\int_{\Xx \times \Yy} g(x,y) \d( \mu\otimes\nu)(x,y) = 
	\int_{\Xx} \int_\Yy g(x,y) \d\mu(x)\d\nu(y). 
}
\end{defn}

\begin{prop}[Lipschitzness of tensorization]\label{prop-tensorization}
	One has, for $(\mu,\mu',\nu,\nu') \in \Mm(\Xx)^2 \times \Mm(\Yy)^2$, 
	\eq{
		\Wass_{\Xx \times \Yy}( \mu \otimes \nu,  \mu' \otimes \nu' ) \leq \Wass_\Xx(\mu,\mu') + \Wass_\Xx(\nu,\nu')
	}
\end{prop}

\begin{proof}
	One has
	\eq{
	\begin{split}
		 &\Wass_{\Xx \times \Yy}( \mu \otimes \nu,  \mu' \otimes \nu' )  \\
		&= \umax{\Lip(g)\leq 1}
			\int_{\Xx \times \Yy} g(x,y) [ \d\mu(x)\d\nu(y)-\d\mu'(x)\d\nu'(y) ] \\
		& = 
		\umax{\Lip(g)\leq 1}
		\int_\Xx \int_\Yy g(x,y)[\d\nu(y)-\d\nu'(y)]\d\mu(x) \\
		& +   
		\int_\Yy \int_\Xx g(x,y)[\d\mu(x)-\d\mu'(x)]\d\nu(y),
	\end{split}
	}
	hence the result.
\end{proof}

%%% Integration.
\paragraph{\underline{Integration.}}
Integration helps agglomerate local information and enforce permutation invariance or equivariance.
\begin{defn}[Integration]
For $f \in \Cc(\Zz \times \Xx; \Yy=\RR^d)$, and $\mu \in \Mm(\Xx)$ we denote
\eq{
	f[\cdot,\mu] \eqdef \int_{\Xx} f(\cdot, x) \d \mu(x) : \Zz \rightarrow \Yy.
}
\end{defn}

\begin{prop}[Lipschitzness of integration]\label{prop-lip-integration}
	With some fixed $\zeta \in \Mm_+^1(\Zz)$ and an $\Ll^2$ norm on $\Yy=\RR^d$, one has
	\begin{align*}
		\norm{f[\cdot,\mu] - f[\cdot,\nu]}_{L^2(\zeta)} \leq d \Lip(f) \Wass_\Xx(\mu,\nu).
	\end{align*}
\end{prop}

\begin{proof}
\eq{
\begin{split}
\lvert \lvert f[\cdot,\mu] & - f[\cdot,\nu] \lvert \lvert_{L^2(\zeta)} \\
& = \int_\Zz \lvert \lvert f[\cdot,\mu](z) - f[\cdot,\nu](z) \lvert \lvert_2 \d\zeta(z) \\
& = \int_\Zz \left\lvert \left\lvert \int_\Xx f(z,x) \d(\mu - \nu)(x) \right\lvert \right\lvert_2 \d\zeta(z) \\
& \leq \int_\Zz \left\lvert \left\lvert \int_\Xx f(z,x) \d(\mu - \nu)(x) \right\lvert \right\lvert_1 \d\zeta(z) \\
& = \int_\Zz \sum_{i=1}^d \left\lvert \int_\mathcal{X} f_i(z,x) \d(\mu-\nu)(x) \right\lvert \d\zeta(z) \\
& \leq \sum_{i=1}^d \Lip(f_i) \Wass_\Xx(\mu,\nu) \\
& \leq d \Lip(f) \Wass_\Xx(\mu,\nu)
\end{split}
}
since again, $\frac{f_i}{\Lip(f_i)}$ is 1-Lipschitz, where $f_i$ is the $i$-th component of $f$.
\end{proof}

%%% Convolution.
\begin{rem}[Convolution]
These simple blocks can help build the convolution $\mu \star \nu \in \Mm(\Xx)$ of two measures $(\mu,\nu) \in \Mm(\Xx)^2$ as a composition of a tensorization block and a push-forward block, namely
\eq{
	\mu\star\nu = f_\sharp (\mu\otimes\nu)
	\qwhereq
	f : (x,y) \in \Xx^2 \mapsto x+y \in \Xx.
}
\end{rem}

%%% Elementary Block.
\paragraph{\underline{Elementary Block.}}

Our previously defined elementary block can be rephrased in a \emph{measure} setting as follows:

\begin{defn}[Elementary Block] \label{EBmeasures}
For $\mu \in \Mm(\Xx)$, using previous notations, we define the elementary block $T_f$ on measures as:
\eq{
\begin{split}
T_f : & \Mm(\Xx) \to \Mm(\Yy) \\
& \mu \to f[\cdot, \mu]_\sharp \mu
\end{split}
}
where $f : \Xx \times \Xx \rightarrow \Yy$. 
\end{defn}

\begin{prop}[Elementary Block on Measures]
For $\mu_\ell \in \Mm(\Xx)$, using previous notations, an elementary block computes:
\eq{
\mu_{\ell+1} = T_{f_{\xi_\ell}}(\mu_\ell) \in \Mm(\Yy)
}
where $f_{\xi_\ell} : \Xx \times \Xx \rightarrow \Yy$; which means, for all $g \in \Cc(\Yy)$,
\eq{
\int_\Yy g(y) \d\mu_{\ell+1}(y) = \int_\Xx g \left( \int_\Xx f_{\xi_\ell}(z,x) \d\mu_\ell(x) \right) \d\mu_\ell(z)
}
Moreover,
\begin{itemize}
	\item If $\mu_\ell \in \Mm_+^1(\RR^{q_\ell})$, then we exactly recover definition \ref{defEB} with the random vector $X_\ell$ distributed according to $\mu_\ell$;
	\item If $\mu_\ell = \delta_c$ is a dirac mass on $c \in \RR^{q_\ell}$, then we recover definition \ref{defEB} in the case of a constant vector $X_\ell = c$.
\end{itemize}
\end{prop}

\begin{prop}[Lipschitzness of Elementary Block Map]
For $(\mu,\nu) \in \Mm_+^1(\Xx)^2$ and $f : \Xx \times \Xx \rightarrow \Yy=\RR^d$,
\eq{
\Wass_\Xx(T_f(\mu), T_f(\nu)) \leq d(\Lip(f)+\Lip(f_1))\Wass_\Xx(\mu,\nu)
}
where $\Lip(f_1)$ stands for the Lipschitz constant w.r.t. the first coordinate of $f$; i.e., the elementary block map $T_f$ is $d(\Lip(f)+\Lip(f_1))$-Lipschitz.
\end{prop}

\begin{proof}
Using the fact that $\Wass_\Xx$ is a norm,
\eq{
\begin{split}
\Wass_\Xx(T_f(\mu), T_f(\nu)) \leq & \Wass_\Xx(T_f(\mu),f[\cdot,\nu]_\sharp \mu) \\
& + \Wass_\Xx(f[\cdot,\nu]_\sharp \mu,T_f(\nu)) \\
\leq & \lvert\lvert f[\cdot,\mu]-f[\cdot,\nu] \lvert\lvert_{L^1(\mu)} \\
& + \Lip(f[\cdot,\nu]) \Wass_\Xx(\mu,\nu)
\end{split}
}
by Lipschitzness of the push-forward (see appendix).
Moreover, for $(z_1,z_2) \in \Xx^2$,
\eq{
\begin{split}
\lvert\lvert &f[z_1,\nu]-f[z_2,\nu] \lvert\lvert_1 \\
& = \lvert\lvert \int_\Xx (f(z_1,x)-f(z_2,x))\d\nu(x) \lvert\lvert_1 \\
& = \sum_{i=1}^d \lvert \int_\Xx (f_i(z_1,x)-f_i(z_2,x)) \d\nu(x) \lvert \\
& \leq \sum_{i=1}^d \int_\Xx \lvert f_i(z_1,x)-f_i(z_2,x) \lvert \d\nu(x) \\
& \leq \sum_{i=1}^d \Lip(f_{1,i}) \lvert\lvert z_1 - z_2 \lvert\lvert_1 \\
& \leq d \Lip(f_1) \lvert\lvert z_1 - z_2 \lvert\lvert_1 \\
\end{split}
}
Hence $\Lip(f[\cdot,\nu]) \leq d \Lip(f_1)$. In addition, Lipschitzness of integration (see appendix) yields:
\eq{
\begin{split}
\Wass_\Xx(T_f(\mu), T_f(\nu)) \leq & d \Lip(f) \Wass_\Xx(\mu, \nu) \\
& + d \Lip(f_1) \Wass_\Xx(\mu,\nu) \\
\end{split}
}
\end{proof}

\begin{rem}[Conditional Push-forwards]
Contrary to a constant map of the form $f_\sharp\mu$, the integration step in $T_f(\mu) = f[\cdot,\mu]_\sharp \mu$ allows to design a push-forward $f[\cdot,\mu]$ that depends on the input measure $\mu$, which is more flexible and increases the richness of the elementary block. Indeed, $f[\cdot,\mu]$ enables us to capture pairwise interactions between points of the input measure $\mu$.
\end{rem}
